# Supplementary material for: VACSEN: A Visualization Approach for Noise Awareness in Quantum Computing
Source: arXiv:2207.14135 source file (2022-07-28)
Supplement: Supplementary file 1 [file appendix.tex]

\section{Overview of All Quantum Computers' Noise}

In Section \ref{subsec:case_2}, we described the comparison of the noise of three quantum computers, \textit{i.e.,} \textit{ibm\_perth}, \textit{ibmq\_manila}, and \textit{ibmq\_lima}. In this section, we briefly introduce the overview of all available quantum computers' noise, which are the attributes of qubit readout error, qubit T1 time, qubit T2 time, and quantum gates.
The time range and interval are the same as the settings in Case Study \uppercase\expandafter{\romannumeral 1} (\textit{i.e.,} seven days and one day, respectively).

As shown in Fig. \ref{fig:apdix_1}  there are nine out of 24 quantum computers available on March-3-2022. Among them, Computer \textit{ibmq\_armonk} has only one qubit, Computer \textit{ibm\_lagos}, \textit{ibm\_perth}, \textit{ibmq\_jakarta} have seven qubits, and other five quantum computers have five qubits. 

For the noise of qubit error rate (Fig. \ref{fig:apdix_1} \component{A}), four quantum computers have stable and high performance, such as \textit{ibm\_lagos}, \textit{ibm\_perth}, \textit{ibmq\_manila}, and \textit{ibmq\_quito}, while the qubits in other quantum computers are noisy regarding the readout error, as indicated by the number of red circles. For the noise of T1 time (Fig. \ref{fig:apdix_1} \component{B}),  \textit{ibm\_perth} and \textit{ibmq\_manila} are much better than other quantum computers regarding the T1 noise, while \textit{ibmq\_belem} and \textit{ibmq\_lima} are the noisiest quantum computers on March-5-2022. The other quantum computers have an intermediate noise for T1 time. 
However, for another noise of decoherence time, \textit{i.e.,} T2 time, a different noise pattern could be observed in Fig. \ref{fig:apdix_1} \component{C}. \textit{ibmq\_jakarta} and \textit{ibmq\_manila} are much noisier than other quantum computers, as indicated by the number of large red circles.
Thus, the user and we found that the noise pattern can be totally different for a quantum computer.
Moreover, we can easily find that the queuing numbers of quantum computers vary on the day of execution. Considering the quantum algorithm to be executed, selecting an appropriate quantum computer concerning the noise type and the corresponding magnitude according to the scale of the quantum algorithm is important for the fidelity of the execution results and the cost of time.
\toolName\ integrates the above factors and informs the users of the noise and properties of all quantum computers via the proposed circuit-like design, making it more effective and time-saving.

\begin{figure*}[b]
\centering
\includegraphics[width=0.9\linewidth]{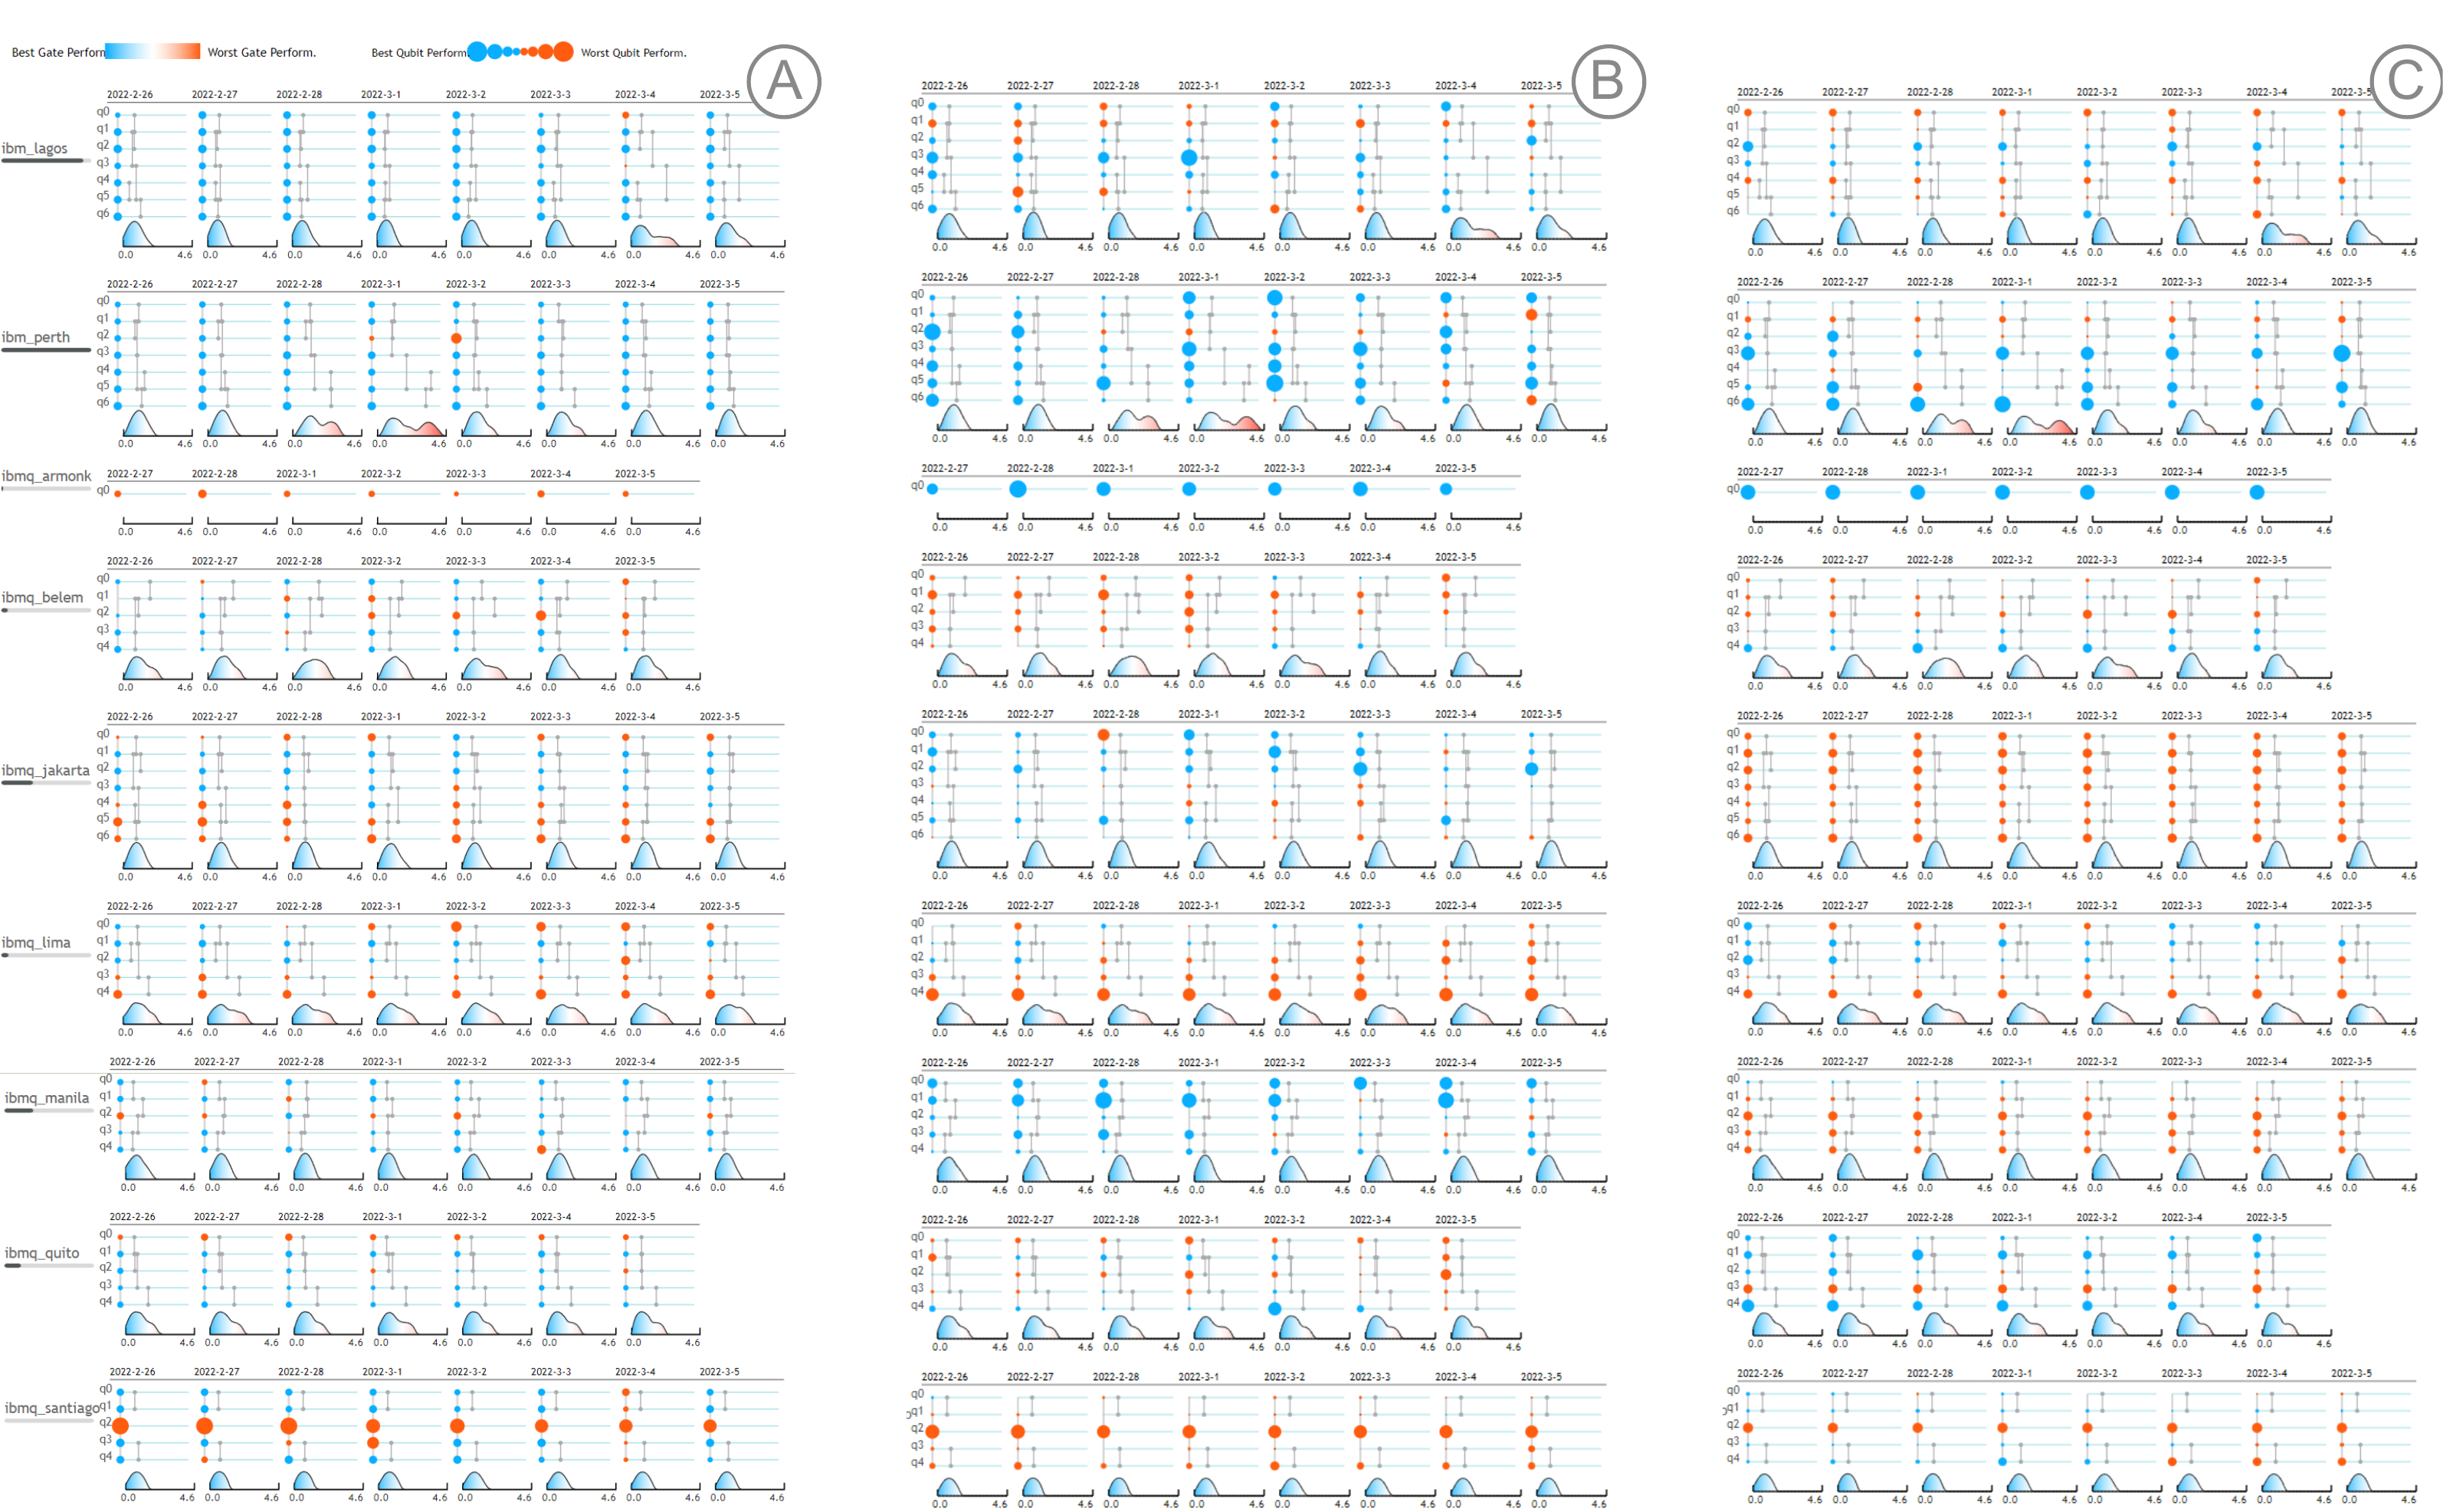}
\caption{Noise awareness for all quantum computers in the IBM Q quantum computing platform. The calibration data was profiled on March-3-2022. The account is under ``IBM Quantum Research'' hub.}
\label{fig:apdix_1}
\end{figure*}

\section{Fidelity of the Execution Result}

In Section \ref{subsec:dataset}, we introduced the dataset for driving \toolName. The last step for executing a quantum algorithm is visualizing the fidelity of the execution result, which is used for validating the previous selection of quantum computers and compiled circuits. In this section, we introduce the approach for fidelity calculation.

We extract the execution results of a quantum algorithm from the remote quantum computing platform and further calculate the fidelity in the processing module.
% need to extract all instructions of all compiled circuits, etc. Specifically, every time the selected computer launches the compilation, our system would  (\textbf{R4}). After selecting the preferred circuit based on the visualization system, the selected circuit would be delivered back to the quantum computer and then executed (\textbf{R5, R6}). 
% The instruction data contains. 
% Besides, we use multiple criteria(\textit{i.e.,} depth of circuit, qubit quality scores, and gate quality scores) for portraying circuits to support the initial filtering for the potential compiled circuit (\textbf{R5}). 
% Users could inspect and compare each circuit via the quality-awareness visualization system.
Followed by the methodology proposed by prior work~\cite{resch2020day, gokhale2020optimized, wille2019mapping}, we use  Hellinger distance~\cite{luo2004informational} for the fidelity calculation.

\begin{equation}
\label{equation:5}
Fidelity = (1-H^2)^2,
\end{equation}

where $H$ is the Hellinger distance~\cite{luo2004informational}. For two probabilities distributions $P = (p_1, ..., p_k)$ and $Q = (q_1, ..., q_k)$, their Hellinger distance is defined as:

\begin{equation}
\label{equation:6}
H(P, Q) = \frac{1}{\sqrt{2}}\sqrt{\sum^k_{i=1}{(\sqrt{p_i} - \sqrt{q_i})^2}}.
\end{equation}

\section{Post-execution Analysis}
In Section \ref{sec:tech}, we explained the Probability Distribution View, which is for the execution result analysis. Through our interview with five experts in quantum computing, they suggested that it is crucial for quantum computing users to get the execution result from \toolName. Given that the execution result is the probability distribution for all possible states (\textit{e.g.}, 00, 01, 10, 11 for a 2-qubit quantum circuit), the total number for all states is determined by the shot number (\textit{e.g.}, 1000 in Case Study \uppercase\expandafter{\romannumeral 1} and Case Study \uppercase\expandafter{\romannumeral 2}). As shown in Fig. \ref{fig:apdix_2}, the grouped bar charts visualize the state distribution of the result, where the blue bars denote the ideal noise-free result generated by the Simulator ``\textit{AerSimulator}'', and the red bars represent the actual experiment results with noise.

\begin{figure}[t]
\centering
\includegraphics[width=0.9\linewidth]{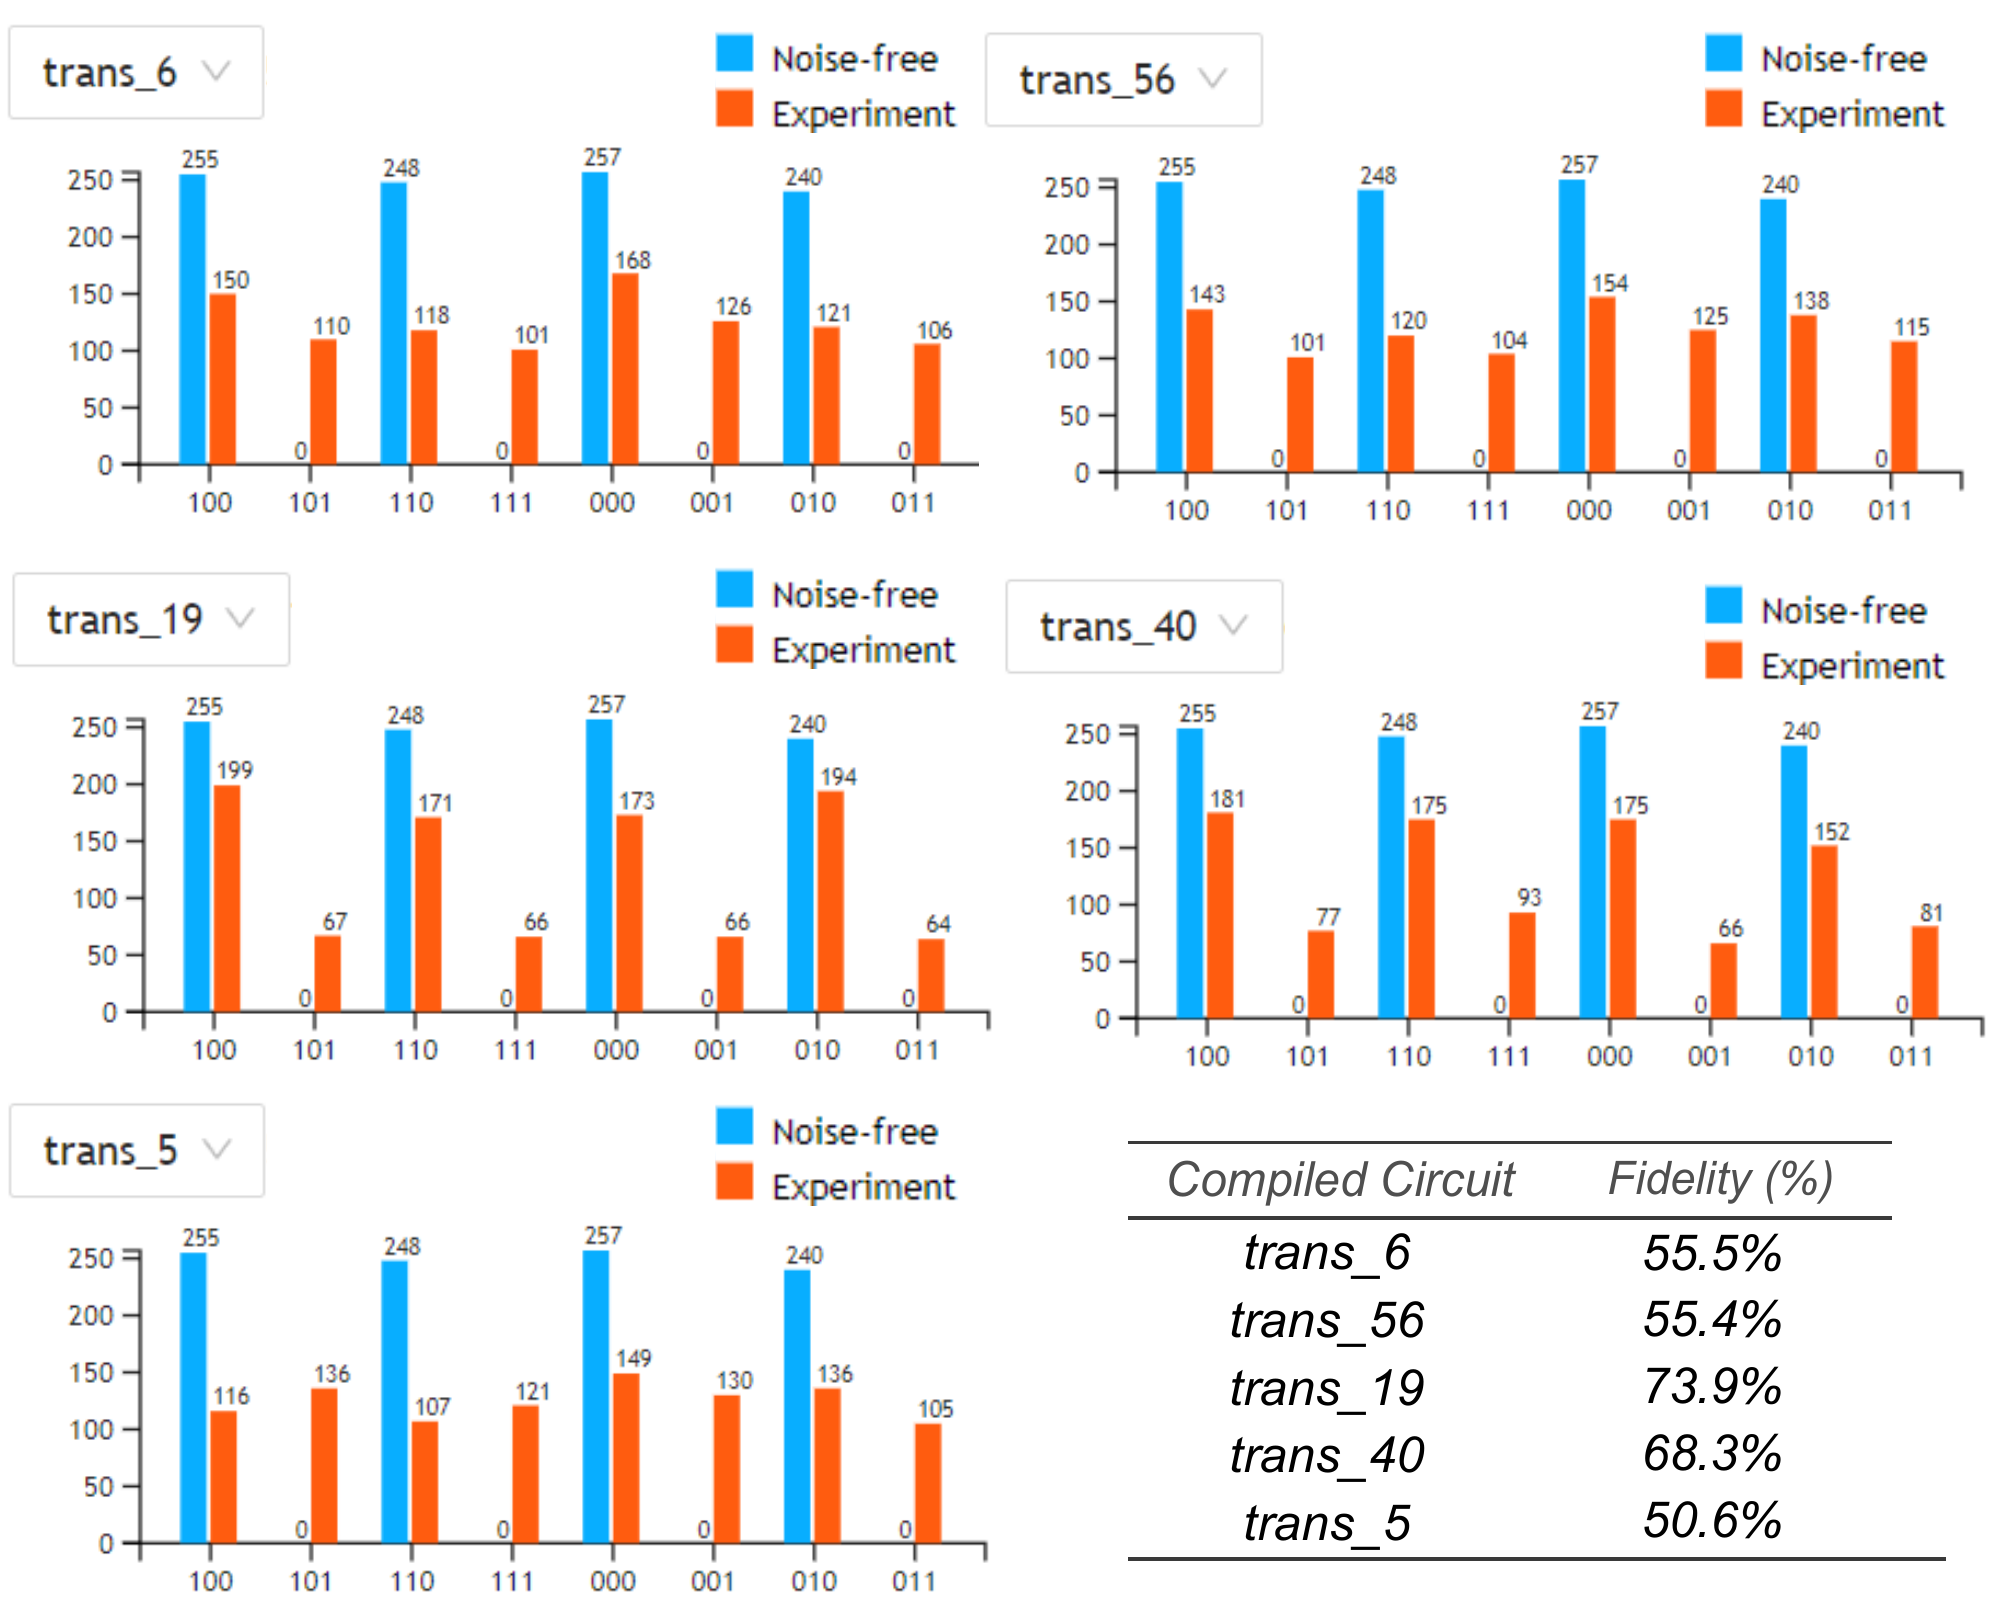}
\caption{Probability Distribution views and the corresponding fidelity.}
\label{fig:apdix_2}
\end{figure}

For example, as shown in Fig. \ref{fig:apdix_2}, the five Probability Distribution Views were the results of the five compiled circuits selected for the in-depth comparison Case Study \uppercase\expandafter{\romannumeral 2}. The blue bars represent the ideal state distribution for the given \textit{Shor-15-Qiskit} algorithm, which has four theoretical states in the noise-free condition (\textit{i.e.,} \textit{100}, \textit{110}, \textit{000}, \textit{010}).
However, the actual result has eight states as some qubits had an erroneous flip, one of the noise sources. 
Thus, some qubits generated a bias compared to the ideal state.

The table in Fig. \ref{fig:apdix_2} shows the fidelity of each compiled circuits. Specifically, Circuit \textit{trans\_19} generated the best result with the highest fidelity (\textbf{73.9\%}), while Circuit \textit{trans\_5} was with the least fidelity (\textbf{50.6\%}). The fidelity difference between the two compiled circuits is over 20\% in this case, which is significantly large and can not be ignored.
Meanwhile, through the Probability Distribution View, one of our collaborators hints that Figure \ref{fig:apdix_2} confirms that the noise could lead to a erroneous result reading compared with the ideal one.
For example, the shot number of the state ``101'' (\textit{i.e.,} which is 136 shots and not the ideal result) was larger than the number of the theoretical states ``\textit{100}'' and ``\textit{110}'', which are 116 and 107 shots respectively and belong to the ideal result set (\textit{i.e.,} \textit{100}, \textit{110}, \textit{000}, \textit{010}).
The same noisy patterns can also be found in Circuit \textit{trans\_6} and \textit{trans\_56}.
Thus, the above cases prove the importance of making the users aware of noise in the compiled circuits and avoid the noisy circuits before the execution, which is exactly one of the major advantages of \toolName.

\section{Explanation of Equation 3}

\modifyRed{In Section \ref{subsec:equation3}, we define the calculation of overall scores $S$ as follows:}

\begin{equation}
\label{equation:5}
S = \modifyRed{(}\frac{\sum_{i=1}^{N}{C_{i} \cdot E_{i}}}{\sum_{i=1}^{N}{C_{i}}}\modifyRed{)}^{\modifyRed{-1}},
\end{equation}

\modifyRed{where $E_{i}$ denotes the error rate of a quantum gate (or qubit), and $C_{i}$ is the usage times of a quantum gate (or qubit). }

% \modify{
% Following Linearly Weighted Moving Average (LWMA)~\cite{lwma}, we propose the above equation to calculate the overall scores $S$.
% Specifically, to summarize the overall performance of a given compiled circuit, we use $N \cdot P_{\varepsilon}$ to represent the gate error or qubit readout error of each quantum gate or qubit regarding the corresponding usage times. We then normalize it with the number of quantum gates or qubits $d$. Finally, we use the reciprocal of the fraction to represent the performance magnitude.
% % the weighted times of each object,
% % \yong{1. What is the relation between LWMA and Ref. \cite{kaneko2015smoothing}? 2. What is ``weighted times of each object''?}
% %  the overall scores of a compiled circuit regarding the implementation times of qubits or quantum gates and their noise levels.
%  }

\begin{figure}[t]
\centering
\includegraphics[width=0.9\linewidth]{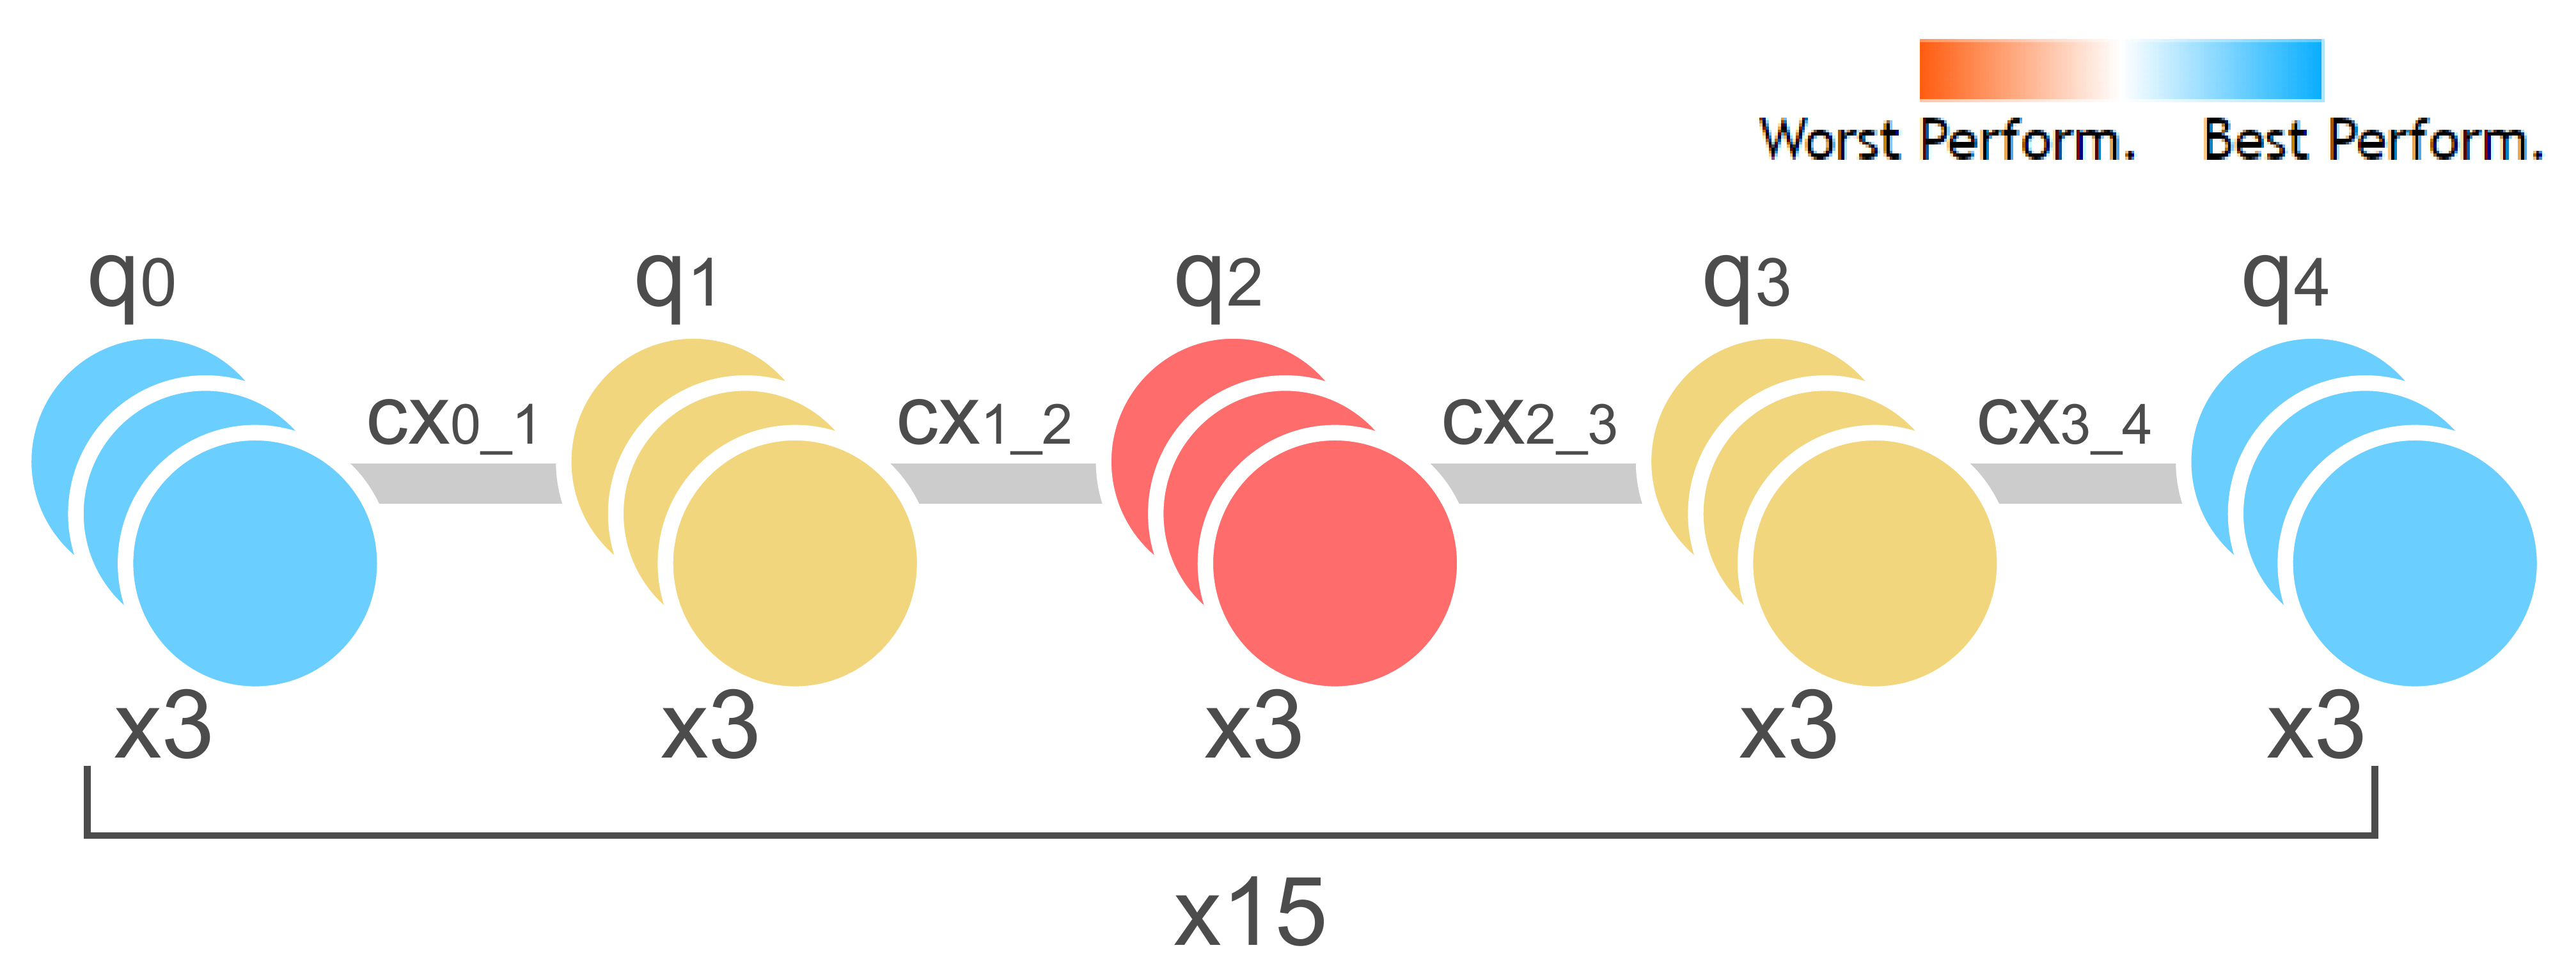}
\caption{\modifyRed{A compiled circuit implemented on a certain quantum computer. Each qubit is implemented multiple times.}}
\label{fig:apdix_3}
\end{figure}

\modifyRed{For example, Fig. \ref{fig:apdix_3} is a compiled circuit implemented on a certain quantum computer which has 5 qubits. Each qubit is implemented 3 times to form the compiled circuit. Assume that the qubit readout error of the five qubits are $10\%, 50\%, 90\%, 50\%, 10\%$, the overall scores $S$ can be calculated as follows:}

\begin{equation}
\label{equation:5}
S = (\frac{3 \times 10\% + 3 \times 50\% + 3 \times 90\% + 3 \times 50\% + 3 \times 10\%}{15})^{-1}.
\end{equation}

\modifyRed{We use the above equation to calculate the overall scores of the qubits. Similarly, we could use the equation to calculate the quantum gates' overall scores. Note that for some small-scale quantum algorithms, some physical qubits or quantum gates may not be implemented for a certain complied circuit.}
